# Supplementary material for: Dual Strategies for Test-Time Adaptation
Source: arXiv:2604.17542 source file (2026-04-19)
Supplement: Supplementary file 1 [file X_suppl.tex]

\clearpage
\setcounter{page}{1}
\maketitlesupplementary

\setcounter{section}{0}

\setcounter{table}{0}
\setcounter{figure}{0}

\section{Theoretical Justification for DualTTA}

In the main paper, we introduced \textbf{DualTTA}, whose core idea is to (i) construct two sample sets, $\mathcal{D}^+$ and $\mathcal{D}^-$, and (ii) adapt the model using different objectives on these sets. For $\mathcal{D}^+$, we minimize prediction entropy to reinforce confident decisions, whereas for $\mathcal{D}^-$, we maximize entropy to suppress overly confident but incorrect predictions. The intuition is that samples in $\mathcal{D}^+$ are those the classifier is \emph{likely} to classify correctly, while those in $\mathcal{D}^-$ are \emph{likely} to be misclassified; hence we referred to them as ``likely-correct'' and ``likely-incorrect'' samples, respectively. However, we have not yet formally shown that $\mathcal{D}^+$ and $\mathcal{D}^-$ indeed correspond to samples with high and low correctness likelihoods. In this section, we state a theorem establishing this property and then provide its detailed proof.\\
As:

%In the main paper, we have proposed DualTAA. Our main idea is: first, construct two set of samples $\mD^+$ and $\mD-$, and second, use the samples in these two sets to adapt the classifier. For the former set, we have propose to minimize the entropy of the classifier on the samples of this set, and on the latter one, we have propose to maximize the entropy. Our rationale is that the samples in $\mD^+$ are the ones that the classifier is likely to classify correctly, so that we should reinforce the classificantion confidence of the classifier. Inversely, the samples in $\mD^-$ are the ones that the classifier is likely to classify incorrectly, so that we should take action to minimize its wrongly overconfident decisions. Given that, we have also given $\mD^+$ and $\mD^-$ the names of likely-correct and likely-incorrect samples. However, we have really given a proof that the samples in $\mD+$ and $\mD^-$ are indeed likely to be classified correctly or incorrectly, respectively. In this section, we first state a theorem that show that is indeed the case, and we then provie the proof for that theorem. 

\myheading{Theorem 1.}
Consider a sample $\mathbf{x}$ with style statistics $(\U, \S)$. Let $\mathbf{x}^{sp}$ denote its semantic-preserving variant obtained by modifying $(\U, \S)$ to $(\U^{sp}, \S^{sp})$, and let $\mathbf{x}^{sa}$ denote its semantic-altering variant produced via a strong augmentation $\mathbf{x}^{sa} = \mathbf{x} + \zeta$ as described in the main paper. \\
Let $\hat{y}(\mathbf{x})$ be the prediction probability of $\x$ and $f(\x)$ be the one-hot label for $\x$, e.g. $f(\x)=\arg \max_c \hat{y}(\x)$, and let $y$ be its (unknown) ground-truth label. Then the probability of $x$ being misclassified is $\text{error}(\x) =  \Pr\!\big(f(\x) \neq y\big)$, and: 
\begin{align}
\Pr\!\big(f(\x) \neq y\big) \;\uparrow\uparrow\;
\frac{\Pr\!\big(f(\mathbf{x}^{sp}) \neq f(\mathbf{x})\big)}
     {\Pr\!\big(f(\mathbf{x}^{sa}) \neq f(\mathbf{x})\big)}.
\end{align}
Here, the symbol $\uparrow\uparrow$ is used to denote a monotonic increasing relationship between the two variables, and $\uparrow\downarrow$ represents the monotonic decreasing relationship.

\myheading{Theorem 2.} 
Consider a sample $\mathbf{x}$ and its variant $\mathbf{x}'=\mT(\x)$ (either a semantic-preserving $\x^{sp}$ or semantic-altering variant $\x^{sa}$ or other transformation). \\
The probability that the model assigns different labels to them is given by $\Pr\!\big(f(\mathbf{x}') \neq f(\mathbf{x})\big)$, and it is proportional to $\text{Diff}(\hat{y}(\mathbf{x}'), \hat{y}(\mathbf{x}))$, where $\hat{y}(\x)$ is the probability prediction and $\text{Diff}(.)$ is the function defined in Equation 2 of the main paper. That is,
\begin{align}
\Pr\!\big(f(\mathbf{x}') \neq f(\mathbf{x})\big) \propto [\text{Diff}(\hat{y}(\mathbf{x}'), \hat{y}(\mathbf{x}))].
\end{align}
\myheading{Corollary.}
For a sample $\x^+ \in \mD^+$ and $\x^- \in \mD^-$, the classification error of $\x^+$ is lower than that of $\x^-$, and there exists a factor $\rho$ such that:
\begin{align}
\text{error}(\x^+) < \rho\frac{\tau^{sp}}{\tau^{sa}} < \text{error}(\x^-),
\end{align}
This corollary follows directly from Theorem 1 and Theorem 2, and from the definitions of $\mD^+$ and $\mD^-$ as presented in the main paper.
\begin{align}
\mD^+ &= \left\{\x \mid 
\mathrm{Diff}(\hat{y}, \hat{y}^{sa}) > \tau^{sa},\ 
\mathrm{Diff}(\hat{y}, \hat{y}^{sp}) < \tau^{sp}
\right\},\nonumber\\
\mD^- &= \left\{\x \mid 
\mathrm{Diff}(\hat{y}, \hat{y}^{sa}) < \tau^{sa},\ 
\mathrm{Diff}(\hat{y}, \hat{y}^{sp}) > \tau^{sp}
\right\},
\end{align}

This corollary justifies the construction of $\mD^+$ and $\mD^-$ and explains why we minimize the entropy for samples in $\mD^+$ while maximizing the entropy for samples in $\mD^-$, as described in the paper.

\section{Theorem Proof}
In this section we present the detailed proofs of the two theorems stated above. Since our theoretical analysis focuses solely on two types of classes—the correct class and the incorrect class for each sample—for clarity and ease of presentation, we restrict the analysis to the binary classification setting with class labels $\{+1,-1\}$
\subsection{Proof of theorem 1}

With the label set $\{+1,-1\}$.
The decision rule can then be written compactly as:
\[
f(\x)=\operatorname{sign}\big(w^\top\phi(\x)\big).
\]
With the assumption above the decision boundary is located at $0$.
% Denote the (real-valued) class scores by $\hat{y}_{+1}(\x)$ and $\hat{y}_{-1}(\x)$. The predicted label is
% \[
% \hat{y}(\x)=\arg\max_{c\in\{+1,-1\}}\hat{y}_c(\x)\in\{+1,-1\}.
% \]
% For a linear (or margin) binary classifier it is convenient to introduce the margin
% \[
% m(\x):= \hat{y}_{+1}(\x)-\hat{y}_{-1}(\x)=w^\top\phi(\x).
% \]
We define $M(\x)$ as the random variable that represents distance between sample $\x$ and the decision boundary 0, then we have:
\[
M(\x) :=|w^\top \phi(\x)|
.\]
Let $F_M$ denote the CDF of $M$, $F_M(t)=Pr(M\le t)$
We consider two types of perturbations applied to $\x$:

\begin{itemize}
    \item \textbf{Style perturbation.}
    Perturbing the feature statistics $(\U,\S)$ to $(\U^{sp},\S^{sp})$ ($\|\U^{sp}-\U\|+\|\S^{sp}-\S\|<\varepsilon$) induces a representation shift
    \[
        \phi(\x^{sp}) \approx \phi(\x) + \Delta_s,
    \]
    whose projection along $w$ has magnitude $s := |w^\top \Delta_s|$.
    The probability of label flip is the probability that the distance to the decision boundary is smaller than the magnitude of the perturbation.
    \[
        \alpha := \Pr\big(f(\x^{sp}) \neq f(\x)\big) =Pr(M\le s)= F_M(s).
    \]

    \item \textbf{Semantic perturbation.}
    Applying a large semantic modification $\x^{sa} = \x + \zeta$ induces a representation shift
    \[
        \phi(\x^{sa}) \approx \phi(\x) + \Delta_{sem},
    \]
    with projected magnitude $S := |w^\top \Delta_{sem}| \gg s$.
    The corresponding label-flip probability is the probability that the distance to the decision boundary is smaller than the magnitude of the perturbation.
    \[
        \beta := \Pr\big(f(\x^{sa}) \neq f(\x)\big)=Pr(M\le S)= F_M(S).
    \]
\end{itemize}

Let the model's prediction error probability for $\x$ be
\[
\text{error}(\x) := \Pr(f(\x) \neq y) = Pr(M<m_0)=F_M(m_0),
\]
where $m_0$ is the threshold under which the classifier fails on $\x$.

The threshold $m_0$ following structural relationships:
\\
1. The threshold $m_0$ increases with the sensitivity to style perturbation:
\[
\exists g(.) ;m_0 = g(s), \qquad g' > 0.
\]
2. The threshold $m_0$ decreases with the sensitivity to semantic perturbation:
\[
\exists \psi(.); m_0 = \psi(S), \qquad \psi' < 0.
\]
We prove that $\text{error}(\x)$ is (i) increasing in $\alpha$ and (ii) decreasing in $\beta$.
\paragraph{(i) $\text{error}(\x)$ increases with $\alpha$.}
Since $\alpha = F_M(s)$ and $F_M$ is strictly increasing, we have $s = F_M^{-1}(\alpha)$.
Thus,
\[
\text{error}
    = F_M(m_0)
    = F_M(g(s))
    = F_M\!\left(g(F_M^{-1}(\alpha))\right).
\]
The composition of three monotone increasing functions ($F_M$, $g$, and $F_M^{-1}$) is increasing; hence
\[
\frac{\partial\text{error}}{\partial\alpha} > 0.
\]
Equivalently,
\begin{equation}
    \text{error(\x)}\uparrow\uparrow\alpha
    \label{eq:alpha}
\end{equation}

\paragraph{(ii) $\text{error}(\x)$ decreases with $\beta$.}

Similarly, since $\beta = F_M(S)$ is increasing in $S$, we have $S = F_M^{-1}(\beta)$, and
\[
\text{error}
    = F_M(m_0)
    = F_M(\psi(S))
    = F_M\!\left(\psi(F_M^{-1}(\beta))\right).
\]
Here $F_M$ and $F_M^{-1}$ are increasing while $\psi$ is strictly decreasing, so the composition is decreasing:
\[
\frac{\partial\text{error}}{\partial\beta} < 0.
\]
Equivalently,
\begin{equation}
    \text{error}(\x)\uparrow\downarrow\beta
    \label{eq:beta}
\end{equation}
From \ref{eq:alpha} and \ref{eq:beta}, we have:
\[
\text{error}\uparrow\uparrow\frac{\alpha}{\beta}
\]
Theorem 1 is proven.
\subsection{Proof of theorem 2}
Let \(\mathbf{x}\) be a fixed input and let $\mathbf{x'}=\mT(\x)$ denote a variant of \(\mathbf{x}\). For binary classification we write the model's probability prediction vectors as
Tie-breaking at \(1/2\) is immaterial for the inequalities below.

For short, we denote
\[
\Delta:=y(\x')-y(\x)=\text{Diff}\big(\hat y(\mathbf{x}'),\hat y(\mathbf{x})\big),\qquad \delta:=\big|y(\x)-\tfrac12\big|.
\]
Let $\mathbb{E}_{\x'\sim \mT(\x)}[|\Delta|]$ denote expectation with respect to the distribution generating $\x'\sim \mT(\x)$, for short we denote as $\mathbb{E}[|\Delta|].$

% For the binary case the paper's difference function reduces to the \(L_1\) distance between probability vectors:
% \[
% \mathrm{Diff}\big(\hat y(\mathbf{x}'),\hat y(\mathbf{x})\big):=\|\hat y(\mathbf{x}')-\hat y(\mathbf{x})\|_1=2|\Delta|.
% \]
% The labels assigned to \(\mathbf{x}\) and \(\mathbf{x}'\) differ exactly when \(p\) and \(p'\) lie on opposite sides of \(1/2\):
% \[
% \{f(\mathbf{x}')\neq f(\mathbf{x})\}\iff (p-\tfrac12)(p'-\tfrac12)<0.
% \]
A label change is that the absolute shift be at least \(\delta\). In other words,
\begin{equation}
    \{\x'\mid f(\mathbf{x}')\neq f(\mathbf{x})\}\subseteq\{\x'\mid\,|\Delta|\ge\delta\,\}.
    \label{eq:bound}
\end{equation}
Similarly, if the probability shift is smaller than $\delta$, the label of $\x$ does not change:
\begin{equation}
    \{\x'\mid f(\mathbf{x}')= f(\mathbf{x})\}\supseteq\{\x'\mid\,|\Delta|\le\delta\,\}.
    \label{eq:bound2}
\end{equation}
We prove that for each $\x$, there exist positive constants $C_1, C_2$ such that:
\[
C_1.\,\mathbb{E}[|\Delta|]\ \le\ \Pr\big(f(\mathbf{x}')\neq f(\mathbf{x})\big)\ \le\ C_2.\mathbb{E}\,[|\Delta|].
\]
\noindent\textbf{Upper bound.}
Take expectation over the randomness of the variant \(\mathbf{x}'\). Using the inclusion in \ref{eq:bound} we obtain:
\begin{align*}
\mathbb{E}\big[|\Delta|\big]
&=\mathbb{E}\big[|\Delta|\cdot\mathbf{1}_{\{f(\mathbf{x}')\neq f(\mathbf{x})\}}\big]+\mathbb{E}\big[|\Delta|\cdot\mathbf{1}_{\{f(\mathbf{x}')=f(\mathbf{x})\}}\big]\\
&\ge \mathbb{E}\big[|\Delta|\cdot\mathbf{1}_{\{f(\mathbf{x}')\neq f(\mathbf{x})\}}\big]\ge \delta\,\Pr\big(f(\mathbf{x}')\neq f(\mathbf{x})\big).
\end{align*}
Rearranging gives:
\begin{equation}
\Pr\big(f(\mathbf{x}')\neq f(\mathbf{x})\big)\le \frac{\mathbb{E}\big[|\Delta|\big]}{\delta}
\label{eq:upperbound}
% =\frac{E\big[\mathrm{Diff}(\hat y(\mathbf{x}'),\hat y(\mathbf{x}))\big]}{2\delta}.
\end{equation}

\noindent\textbf{Lower bound.}
We can decompose the expectation into the following:
\begin{align}
    \mathbb{E}\big[|\Delta|\big]=&\mathbb{E}\big[|\Delta|\mid f(\mathbf{x}')\neq f(\mathbf{x})\big]\Pr(f(\mathbf{x}')\neq f(\mathbf{x}))\nonumber\\
    &+\mathbb{E}\big[|\Delta|\mid f(\mathbf{x}')=f(\mathbf{x})\big]\big(1-\Pr(f(\mathbf{x}')\neq f(\mathbf{x}))\big).
    \nonumber
\end{align}

From \ref{eq:bound2} and the trivial upper bound \(|\Delta|\le 1\), we obtain:
\begin{align}
    \mathbb{E}\big[|\Delta|\big]\le& 1\cdot\Pr(f(\mathbf{x}')\neq f(\mathbf{x}))+\delta\big(1-\Pr(f(\mathbf{x}')\neq f(\mathbf{x}))\big)\nonumber\\
    &=\delta+(1-\delta)\Pr(f(\mathbf{x}')\neq f(\mathbf{x})).
    \nonumber
\end{align}
Hence,
\begin{equation}
    \Pr\big(f(\mathbf{x}')\neq f(\mathbf{x})\big)\ge\frac{\mathbb{E}\big[|\Delta|\big]-\delta}{1-\delta}
    \label{eq:lowerbound}
\end{equation}

% =\frac{\tfrac12E\big[\mathrm{Diff}(\hat y(\mathbf{x}'),\hat y(\mathbf{x}))\big]-\delta}{1-\delta}.

Combining \ref{eq:upperbound} and \ref{eq:lowerbound}, for fixed \(\mathbf{x}\) (hence fixed \(\delta\)), we have:
\begin{equation}
    \frac{\mathbb{E}[|\Delta|]-\delta}{1-\delta}
    \ \le\
    \Pr\big(f(\mathbf{x}')\neq f(\mathbf{x})\big)
    \ \le\
    \frac{\mathbb{E}\big[|\Delta|\big]}{\delta}.
\end{equation}
In particular, whenever \(\delta\) is bounded away from zero there exist positive constants \(C_1,C_2\) depend on fixed $\delta$ such that:
\begin{align}
    C_1.\mathbb{E}_{\x'\sim\mT}[|\Delta|] \le\ \Pr\big(f(\mathbf{x}')\neq f(\mathbf{x})\big)\ \nonumber
    \le\ C_2\,\mathbb{E}_{\x'\sim\mT}[|\Delta|].
\end{align}
Then, for a fixed transformation $\mT(.)$, there exists a constant $C_\mT$, $C_1<C_\mT<C_2$, such that:
\begin{align}
    \Pr\big(f(\mathbf{x}')\neq f(\mathbf{x})\big)=C_{\mT}.|\Delta|.
    \nonumber
\end{align}
Equivalently, with $\Delta=\text{Diff}(\hat y(\mathbf{x}'),\hat y(\mathbf{x}))$,
\begin{align}
    \Pr\big(f(\mathbf{x}')\neq f(\mathbf{x})\big)\propto\mathrm{Diff}(\hat y(\mathbf{x}'),\hat y(\mathbf{x})).
\end{align}
Theorem 2 is proven.
\section{Algorithm Pseudo Code}
Algorithm \ref{alg:dualtta} presents the pseudocode for our proposed DualTTA, which details the selection of low‐entropy samples, partitioning into aligned and misaligned sets, and the subsequent parameter update.
\section{Devices Detail and Latency Analysis}
\subsection{Devices Detail.}
All experiments in this study were conducted on a system equipped with an NVIDIA GeForce RTX 4090 GPU with 24,564 MiB of GPU memory, of which up to 13,664 MiB was utilized during training. The computing environment was configured with NVIDIA driver version 535.183.01, CUDA Toolkit version 12.2, and ran on a Linux operating system. All models were implemented using Pytorch.
\subsection{Latency analysis.}
Table \ref{tab:run-time} presents the results of measuring the time required for adaptation of 50000 samples in our proposed DualTTA and baselines under ImageNet-C, Gaussian noise, and severity level 5 environments. DualTTA achieves the highest performance while requiring less time than SAR and only slightly slower than other baselines.
\begin{table}[t] 
\centering
    \resizebox{0.8\linewidth}{!}{
        \begin{tabular}{l|cc|c}
        \toprule
        Methods & \% adapt &\% correct & GPU time \\ 
        \midrule
        No adapt & x & x &1m 58s \\
        TENT & 100\% & x & 2m 08s \\
        EATA & 28.2\% & 60.1\% & 2m 31s \\
        SAR & 27.2\% & 62.4\% & 4m 19s \\
        DEYO & 31.7\% & 75.9\% & 3m 11s \\ 
        \midrule
        DualTTA & 35.6\% &89.5\% & 4m 11s\\
        \bottomrule
        \end{tabular}%
    }
    \caption{\footnotesize{Data efficiency and runtime evaluation under ImageNet-C, Gaussian noise, and severity level 5.}}
    \label{tab:run-time}
    \end{table}
\section{Hyperparameter Explanation}
\subsection{List of hyperparameters and range of values}
Our proposed DualTTA relies on $4$ essential hyperparameters: content-preserving threshold $\tau^{sp}$, semantic-altering threshold $\tau^{sa}$,normalization factor $\text{Diff}_0$ and trade-off coefficient between the two loss terms $\lambda$, in addition to the parameters introduced in previous works:  normalization factor $\text{Ent}_0=0.4$.

For the range of these hyperparameters, we balance the semantic-preserving and semantic-altering threshold by setting $\tau^{sp}\in [0.6, 0.9]$ and $\tau^{sa}\in[0.2, 0.5]$. Setting $\tau^{sp}$ too low or $\tau^{sa}$ too high causes model-misaligned set $D^-$ to dominate model-aligned set $D^+$, leading the model to focus more on unlearning information from $D^-$ rather than learning from $D^+$. 
% The entropy threshold $\tau_{\text{Ent}}$ is selected in accordance with prior entropy-based adaptation methods, such as TENT and DeYO, which rely on confidence-driven criteria to guide model adaptation. 
To ensure both the non-negativity and numerical balance of the components in Eq.(7), we introduce normalization constants $\text{Diff}_0 \approx \tau^{\text{sp}}$ and $\text{Ent}_0=0.4$. These constants act as scaling factors that stabilize the relative contributions of the entropy and sensitivity-aware terms during optimization. The trade-off coefficient $\lambda$ serves as a balancing factor between two competing objectives in the overall loss function. Specifically, it controls the relative contribution of each loss term---typically one promoting confident predictions (e.g., entropy minimization) and the other enforcing corrective behavior (e.g., entropy maximization or regularization).

\subsection{Performance stability under changes in hyperparameters}
\label{hyper-param}
To assess the sensitivity of our method to these hyperparameters, we conduct an ablation study whose outcomes are presented in Figure 3 of the manuscript (for semantic-preserving threshold $\tau^{sp}$ and semantic-altering threshold $\tau^{sa}$) and Table \ref{tab:impact3} (for Waterbirds) and \ref{tab:impact-ohh} (for Office-Home) of the Supplementary materials (for others). The results indicate that our proposed DualTTA exhibits strong robustness across a range of threshold values, demonstrating that the method does not heavily rely on precise tuning of these hyperparameters to achieve consistent performance.

For generalization, through all the results of the experiment in the main manuscript, we set $\tau^{sp}=0.7,\text{Diff}_0=0.7,\tau^{ca}=0.4$ and $ \lambda=0.5$.

\section{Impact of semantic-preserving positional layer}
In this section, we conduct additional experiments on the ImageNet-C dataset on the placement of the semantic-preserving (style perturbation) layer using two backbones: ResNet50 and ViT-B. In deep learning architectures with $N$ encoder layers, the style-extraction layer $i$ is selected from the range $\left[\frac{N}{4}, \frac{3N}{4}\right]$ to balance abstraction and semantic entanglement. Early layers often lack stylistic detail, while later layers tend to entangle style with class-specific semantics. Therefore, the appropriate range of values to extract style features is $i = [1,3]$ for ResNet (with $N=4$) and $i = [4,9]$ for ViT-B/32 (with $N = 12$). As shown in Figure \ref{fig:style} of the Supplementary Material, varying $i$ within this range has minimal impact on performance, confirming the robustness of the proposed DualTTA framework.

To enhance generalization, we set the semantic-preserving layer position to 1 for the ResNet backbone and 7 for the ViT-B backbone across all the experiments.

\begin{table*}[]
    \begin{minipage}[t]{.48\textwidth}
    \vspace{0pt}
    \centering
    \resizebox{1\textwidth}{!}{
        \begin{tabular}{l|llll}
    \rowcolor[HTML]{C0C0C0} 
    \toprule
     $\text{Ent}_0=$& 0.1 & 0.3 & 0.4 & 0.5 \\ \hline
    \rowcolor[HTML]{ACE5EE} 
    DualTTA & 86.33 & 87.12 & \textbf{88.44} & 88.25 \\ \midrule
    % \rowcolor[HTML]{C0C0C0} 
    %  $\tau^{ca}=$& 0.1 & 0.3 & 0.4 & 0.5 \\ \hline
    % \rowcolor[HTML]{ACE5EE} 
    % DualTTA & 85.89 & 88.14 & \textbf{88.44} & 88.22 \\ \midrule
    \rowcolor[HTML]{C0C0C0} 
     $\text{Diff}_0=$& 0.6 & 0.7 & 0.8 & 0.9 \\ \hline
    \rowcolor[HTML]{ACE5EE} 
    DualTTA & 88.02 & 88.44 & \textbf{88.50} & 88.22 \\ \midrule
    \rowcolor[HTML]{C0C0C0} 
     $\lambda=$& 0.3 & 0.5 & 0.7 & 0.9 \\
    \rowcolor[HTML]{ACE5EE} 
    DualTTA & 88.08 & \textbf{88.44} & 88.02 & 87.12\\
    \bottomrule
    \end{tabular}%
    }
    \captionof{table}{Impact of different hyper-parameters on Waterbirds dataset.}
    \label{tab:impact3}
    \end{minipage}
    \hfill
    \begin{minipage}[t]{.48\textwidth}
    \vspace{0pt}
    \centering
    \resizebox{1\textwidth}{!}{
        \begin{tabular}{l|llll}
    \rowcolor[HTML]{C0C0C0} 
    \toprule
     $\text{Ent}_0=$& 0.1 & 0.3 & 0.4 & 0.5 \\ \hline
    \rowcolor[HTML]{ACE5EE} 
    DualTTA & 59.64 & 61.28 & \textbf{61.51} & 61.34 \\ \midrule
    % \rowcolor[HTML]{C0C0C0} 
    %  $\tau^{ca}=$& 0.1 & 0.3 & 0.4 & 0.5 \\ \hline
    % \rowcolor[HTML]{ACE5EE} 
    % DualTTA & 60.78 & \textbf{61.56} & 61.51 & 61.20 \\ \midrule
    \rowcolor[HTML]{C0C0C0} 
     $\text{Diff}_0=$& 0.6 & 0.7 & 0.8 & 0.9 \\ \hline
    \rowcolor[HTML]{ACE5EE} 
    DualTTA & 61.36 & \textbf{61.51} & 61.44 & 61.47 \\ \midrule
    \rowcolor[HTML]{C0C0C0} 
     $\lambda=$& 0.3 & 0.5 & 0.7 & 0.9 \\
    \rowcolor[HTML]{ACE5EE} 
    DualTTA & 61.35 & \textbf{61.51} & 61.14 & 59.69\\
    \bottomrule
    \end{tabular}%
    }
    \captionof{table}{Impact of different hyper-parameters on Office-Home dataset.}
    \label{tab:impact-ohh}
    \end{minipage}
\end{table*}

\begin{figure*}[t]
    \begin{minipage}[t]{.48\textwidth}
    \vspace{20pt}
    \centering
    \resizebox{1\textwidth}{!}{
        \begin{tabular}{l||cc|cc}
            \toprule
            \multicolumn{1}{c||}{} & \multicolumn{2}{c|}{$\alpha(\textbf{x})$} & \multicolumn{2}{c}{$\beta(\textbf{x})$} \\ \cmidrule{2-5}
            \multicolumn{1}{c||}{\multirow{-2}{*}{Sample weights}} & Office-Home & Waterbirds & Office-Home & Waterbirds \\ \midrule
            Ent+SA+SP & \cellcolor[HTML]{ACE5EE}\textbf{61.51} & \cellcolor[HTML]{ACE5EE}\textbf{88.44} & 58.00 & 84.34 \\
            Ent+SA & 60.08 & 87.33 & 60.58 & 87.28 \\
            Ent+SP & 60.65 & 86.72 & 60.74 & 87.22 \\
            Ent & 58.22 & 85.02 & \cellcolor[HTML]{ACE5EE}\textbf{61.51} & \cellcolor[HTML]{ACE5EE}\textbf{88.44} \\
            \bottomrule
            \end{tabular}%
    }
    \captionof{table}{Impact of sample weighting.}
        \label{tab:weight}
    \end{minipage}
    \hfill
    \begin{minipage}[t]{.5\textwidth}
        \vspace{0pt}
        \centering
        \subfloat[ResNet50]{\includegraphics[width=0.48\linewidth]{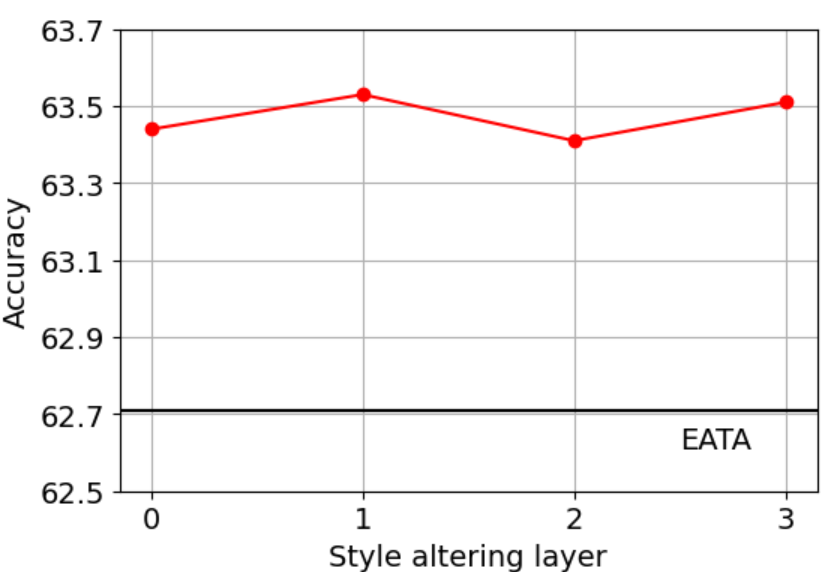}}
        \hfill
        \subfloat[ViT-B]{\includegraphics[width=0.48\linewidth]{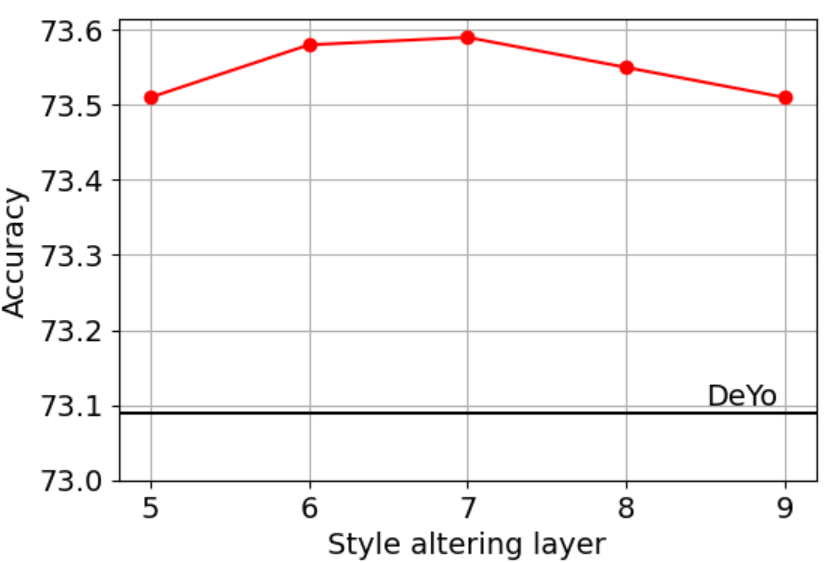}}
        \caption{Performance of proposed method DualTTA with different semantic-preserving positional layer.}
        \label{fig:style}
    \end{minipage}
\end{figure*}

\begin{table*}[t]
\centering
\resizebox{1\linewidth}{!}{%
\begin{tabular}{l|ccc|
>{\columncolor[HTML]{96FFFB}}c |ccc|
>{\columncolor[HTML]{96FFFB}}c |ccc|
>{\columncolor[HTML]{96FFFB}}c |ccc|
>{\columncolor[HTML]{96FFFB}}c |
>{\columncolor[HTML]{FFCE93}}c }
\toprule
\rowcolor[HTML]{D9D9D9} \multicolumn{18}{c}{\textbf{Office-Home:} Art (A), Clipart (C), Product (P), Realworld (R)} \\
\midrule
& \multicolumn{3}{c|}{\textbf{Train domain $\rightarrow$ Test domain}} & \cellcolor[HTML]{68CBD0}\textbf{Train : A} 
& \multicolumn{3}{c|}{\textbf{Train domain $\rightarrow$ Test domain}} & \cellcolor[HTML]{68CBD0}\textbf{Train : C} 
& \multicolumn{3}{c|}{\textbf{Train domain $\rightarrow$ Test domain}} & \cellcolor[HTML]{68CBD0}\textbf{Train : P} 
& \multicolumn{3}{c|}{\textbf{Train domain $\rightarrow$ Test domain}} & \cellcolor[HTML]{68CBD0}\textbf{Train : R} 
& \cellcolor[HTML]{F8A102} \\ 
\cmidrule{2-17}
\multirow{-2}{*}{Methods} & A$\rightarrow$C & A$\rightarrow$P & A$\rightarrow$R & Mean 
& C$\rightarrow$A & C$\rightarrow$P & C$\rightarrow$R & Mean 
& P$\rightarrow$A & P$\rightarrow$C & P$\rightarrow$R & Mean 
& R$\rightarrow$A & R$\rightarrow$C & R$\rightarrow$P & Mean 
& \multirow{-2}{*}{\cellcolor[HTML]{F8A102}\textbf{Avg}} \\ 
\midrule
ResNet50-BN & 43.16 & 60.13 & 72.23 & 58.51 & 53.61 & 61.05 & 65.23 & 59.96 & 52.45 & 42.27 & 72.71 & 55.81 & 64.07 & 47.49 & 75.26 & 62.28 & 59.14 \\
+TENT & 47.08 & 62.83 & 72.89 & 60.93 & 55.17 & 63.17 & \textbf{\color[HTML]{FE0000}66.12} & 61.49 & 54.39 & 45.18 & \textbf{\color[HTML]{FE0000}73.58} & 57.72 & 65.27 & 51.00 & 76.28 & 64.18 & 61.08 \\
+SAR & 44.74 & 61.00 & 72.37 & 59.37 & 54.47 & 62.09 & 65.96 & 60.84 & 53.85 & 42.13 & 72.30 & 56.09 & 65.22 & 48.25 & 75.49 & 62.99 & 59.82 \\
+EATA & 35.60 & 52.29 & 67.98 & 51.96 & 50.43 & 52.83 & 60.16 & 54.47 & 48.95 & 28.55 & 69.38 & 48.96 & 61.52 & 32.33 & 68.12 & 53.99 & 52.34 \\
+DEYO & 43.96 & 61.03 & 71.33 & 58.77 & 53.98 & 61.14 & 65.16 & 60.09 & 53.11 & 41.42 & 71.61 & 55.38 & 64.40 & 46.69 & 75.13 & 62.07 & 59.08 \\
\midrule
+\textbf{DualTTA} & \textbf{\color[HTML]{FE0000}49.98} & \textbf{\color[HTML]{FE0000}63.12} & \textbf{\color[HTML]{FE0000}72.93} & \textbf{\color[HTML]{FE0000}62.01} & \textbf{\color[HTML]{FE0000}55.67} & \textbf{\color[HTML]{FE0000}63.17} & 65.99 & \textbf{\color[HTML]{FE0000}61.61} & \textbf{\color[HTML]{FE0000}54.35} & \textbf{\color[HTML]{FE0000}46.19} & 73.28 & \textbf{\color[HTML]{FE0000}57.94} & \textbf{\color[HTML]{FE0000}65.64} & \textbf{\color[HTML]{FE0000}51.30} & \textbf{\color[HTML]{FE0000}76.50} & \textbf{\color[HTML]{FE0000}64.48} & \textbf{\color[HTML]{FE0000}61.51} \\
\midrule
\rowcolor[HTML]{D9D9D9} \multicolumn{18}{c}{\textbf{PACS:} Art (A), Cartoon (C), Photo (P), Sketch (S)} \\
\midrule
& \multicolumn{3}{c|}{\textbf{Train domain $\rightarrow$ Test domain}} & \cellcolor[HTML]{68CBD0}\textbf{Train : A} 
& \multicolumn{3}{c|}{\textbf{Train domain $\rightarrow$ Test domain}} & \cellcolor[HTML]{68CBD0}\textbf{Train : C} 
& \multicolumn{3}{c|}{\textbf{Train domain $\rightarrow$ Test domain}} & \cellcolor[HTML]{68CBD0}\textbf{Train : P} 
& \multicolumn{3}{c|}{\textbf{Train domain $\rightarrow$ Test domain}} & \cellcolor[HTML]{68CBD0}\textbf{Train : S} 
& \cellcolor[HTML]{F8A102} \\ 
\cmidrule{2-17}
\multirow{-2}{*}{Methods} & A$\rightarrow$C & A$\rightarrow$P & A$\rightarrow$S & Mean 
& C$\rightarrow$A & C$\rightarrow$P & C$\rightarrow$S & Mean 
& P$\rightarrow$C & P$\rightarrow$A & P$\rightarrow$S & Mean 
& S$\rightarrow$C & S$\rightarrow$P & S$\rightarrow$A & Mean 
& \multirow{-2}{*}{\cellcolor[HTML]{F8A102}\textbf{Avg}} \\ 
\midrule
ResNet50-BN & 75.73 & 96.65 & 70.20 & 80.86 & 81.98 & 95.21 & 73.71 & 83.63 & 64.29 & 78.32 & 46.40 & 63.00 & 68.64 & 57.78 & 59.13 & 61.85 & 72.34 \\
+TENT & 77.39 & 96.89 & 72.79 & 82.36 & 84.96 & 95.49 & 78.19 & 86.28 & 67.75 & 78.81 & 48.39 & 64.98 & 70.44 & 58.32 & 60.89 & 63.22 & 74.96 \\
+SAR & 76.92 & 96.89 & 71.72 & 81.84 & 83.30 & 95.45 & 73.81 & 84.19 & 65.87 & 77.88 & 47.52 & 63.76 & 70.01 & 58.26 & 61.47 & 63.25 & 73.26 \\
+EATA & 75.60 & 97.25 & 70.09 & 80.98 & 83.35 & 94.85 & 73.43 & 83.88 & 65.36 & 78.37 & 46.70 & 63.48 & 68.13 & 57.72 & 58.69 & 61.52 & 72.46 \\
+DEYO & \textbf{\color[HTML]{FE0000}78.24} & \textbf{\color[HTML]{FE0000}97.49} & 67.93 & 81.22 & 85.89 & 95.27 & 78.37 & 86.51 & \textbf{\color[HTML]{FE0000}71.33} & \textbf{\color[HTML]{FE0000}79.35} & 52.97 & 67.88 & 71.72 & 59.20 & \textbf{\color[HTML]{FE0000}64.01} & \textbf{\color[HTML]{FE0000}65.04} & 75.16 \\
\midrule
+\textbf{DualTTA} & 77.90 & 97.37 & \textbf{\color[HTML]{FE0000}72.59} & \textbf{\color[HTML]{FE0000}82.62} & \textbf{\color[HTML]{FE0000}86.67} & \textbf{\color[HTML]{FE0000}95.51} & \textbf{\color[HTML]{FE0000}78.64} & \textbf{\color[HTML]{FE0000}86.94} & 70.92 & 79.00 & \textbf{\color[HTML]{FE0000}59.99} & \textbf{\color[HTML]{FE0000}69.90} & \textbf{\color[HTML]{FE0000}72.12} & \textbf{\color[HTML]{FE0000}59.22} & 62.55 & 64.63 & \textbf{\color[HTML]{FE0000}76.02} \\
\bottomrule
\end{tabular}%
}
\caption{Detail performance of DualTTA on Office-Home and PACS datasets.}
\label{tab:detail-oh-pacs}
\end{table*}

\section{Impact of sample weighting factor}
% \begin{table}[]
%         \vspace{0pt}
%         \centering
%         \resizebox{1\linewidth}{!}{%
%             \begin{tabular}{l||cc|cc}
%             \toprule
%             \multicolumn{1}{c||}{} & \multicolumn{2}{c|}{$\alpha(\textbf{x})$} & \multicolumn{2}{c}{$\beta(\textbf{x})$} \\ \cmidrule{2-5}
%             \multicolumn{1}{c||}{\multirow{-2}{*}{Sample weights}} & Office-Home & Waterbirds & Office-Home & Waterbirds \\ \midrule
%             Ent+CA+SA & \cellcolor[HTML]{ACE5EE}\textbf{61.51} & \cellcolor[HTML]{ACE5EE}\textbf{88.44} & 58.00 & 84.34 \\
%             Ent+CA & 60.08 & 87.33 & 60.58 & 87.28 \\
%             Ent+SA & 60.65 & 86.72 & 60.74 & 87.22 \\
%             Ent & 58.22 & 85.02 & \cellcolor[HTML]{ACE5EE}\textbf{61.51} & \cellcolor[HTML]{ACE5EE}\textbf{88.44} \\
%             \bottomrule
%             \end{tabular}%
%         }
%         \captionof{table}{Impact of sample weighting.}
%         \label{tab:weight}
%     \end{table}
To study the effectiveness of using the reliability weight $\alpha(\textbf{x})$ and $\beta(\textbf{x})$, which consists of three main components: Ent, Semantic-Preserving weight (SP), and Semantic-Altering weight (SA), we analyze the impact of these parameters when tested on the Waterbirds and Office-Home datasets with varying weight configurations. The results presented in \Tref{tab:weight} indicate that the model achieves the best performance when $\alpha(\textbf{x})$ incorporates entropy weight, semantic-preserving weight (SP), and semantic-altering weight (SA), while $\beta(\textbf{x})$ utilizes only the entropy weight. The reason is that model-aligned samples are filtered based on three factors: entropy, semantic-altering, and semantic-preserving, meaning their reliability depends on all three criteria. Meanwhile, $\beta(\textbf{x})$ serves as a coefficient that helps the model forget the knowledge from model-misaligned samples. However, if $\beta(\textbf{x})$ is too large, the model may prioritize forgetting over learning from model-aligned samples.
\section{Further experiment results}
\subsection{Real and unknown domain shift}

DualTTA as well as other TTA methods are designed to perform test-time adaptation (TTA) to reduce the domain discrepancy between training and testing data. In the main paper, we demonstrated its advantages over existing TTA methods through controlled experiments across multiple datasets exhibiting spurious correlations, domain shifts, or simulated corruptions such as noise, blur, or adverse weather conditions. In this experiment, we evaluate DualTTA in a more realistic setting where domain shift is assumed but neither its nature nor its extent is known a priori. To do so, we seek a dataset with many classes, each containing multiple images with varying numbers of object instances. Our goal is to assess whether TTA can still improve performance in such a challenging scenario, where the number of classes is large and each class exhibits significant intra-class variation. Unlike previous controlled settings, here we simply test whether a pretrained classifier can be effectively adapted at test time to improve accuracy.

Given this purpose, we use FSC147~\cite{m_Ranjan-etal-CVPR21}, a dataset originally developed for visual object counting. This dataset is ideal for our evaluation because it contains 147 object categories, each with a diverse number of annotated instances. We construct a new classification benchmark by cropping each annotated object (using the provided bounding boxes) to form individual image samples.

Because this benchmark involves a large number of categories, it is natural to adopt an open-vocabulary classifier. To examine whether DualTTA is compatible with such models, we use the CLIP ViT-B/32 model (public weights) for all experiments. For each cropped image, we extract an image embedding using CLIP's vision encoder. For each class $C$ in the 147 categories, we construct a text embedding using the prompt ``A photo of \textless C\textgreater''. Classification is then performed by assigning each test image to the class whose text embedding has the highest correlation with the image embedding. The text embeddings remain frozen throughout, while the image embeddings are adapted at test time.

\Tref{tab:fsc147} reports the performance of DualTTA and competing TTA baselines. Most TTA methods (except TENT) improve the accuracy of the base classifier, demonstrating the feasibility and usefulness of applying TTA to open-vocabulary classification under unknown domain shift. DualTTA achieves more than a 2\% improvement over the no-adaptation baseline---a substantial gain given the difficulty of the task, which requires selecting a correct label among 147 classes (with extremely low chance performance). Among all evaluated TTA methods, DualTTA achieves the best performance, surpassing other baselines by a significant margin.

\begin{figure*}
    \centering
    \includegraphics[width=0.9\linewidth]{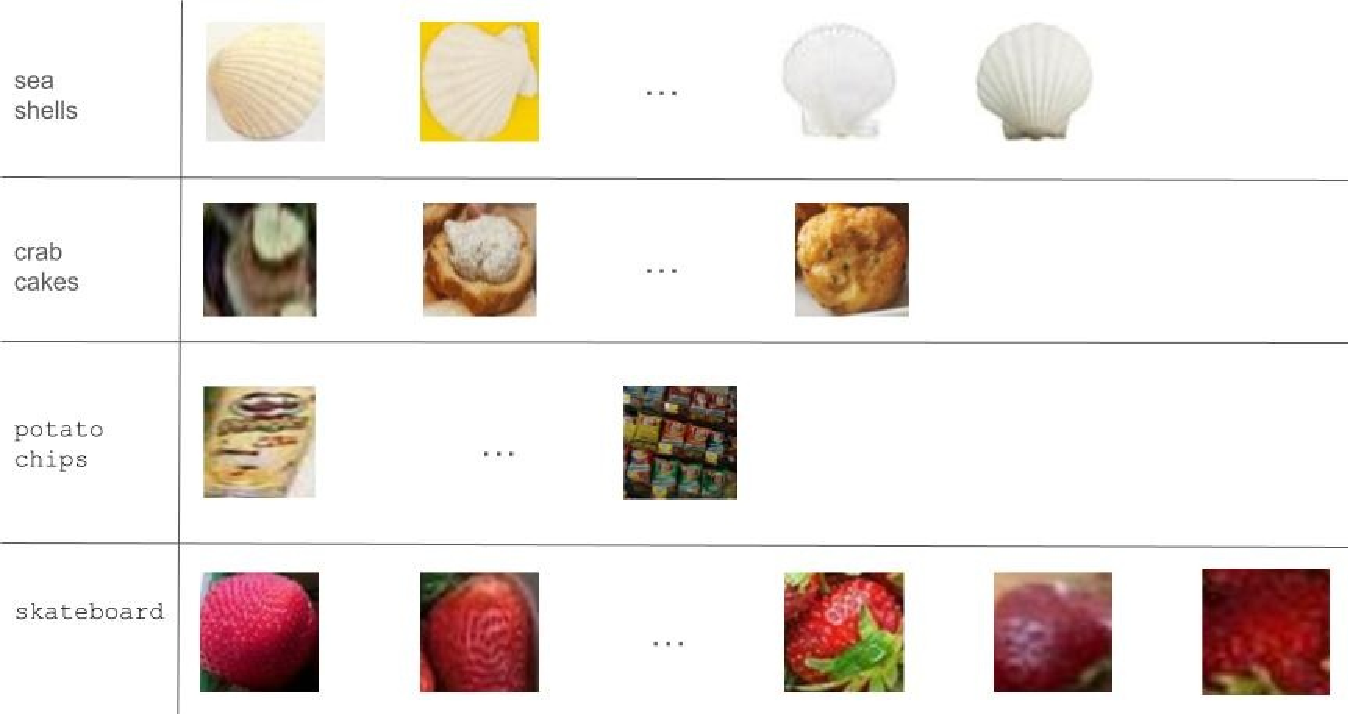}
    \caption{Examples of objects cropped from images in the FSC147 dataset. The number of objects per class differs significantly, resulting in a highly imbalanced dataset. Moreover, the varying sizes of the bounding boxes require resizing them to a unified resolution, which causes some images to become blurred or degraded in quality. }
    \label{fig:fsc147}
\end{figure*}

%Since no pretrained classification model is available for this dataset, we adopt the CLIP model for our experiments. Each class is associated with the prompt “A photo of …” and encoded using CLIP’s text encoder to obtain fixed text embeddings. These text features are kept frozen and aligned with the image features extracted by encoding each cropped image using the vision encoder. Classification is then performed by comparing the image embeddings against the fixed class embeddings. We use the public ViT-B/32 weights of CLIP for all experiments on this dataset.

\begin{center}
\begin{tabular}{lc}
\toprule
Methods & Acc \\
\midrule
Pre-trained CLIP-based classifier (no adaptation) & 17.38 \\
TENT & 14.13 \\
EATA & 18.55 \\
SAR & 17.91 \\
DEYO & 18.95 \\
%\midrule
%DualTTA W/O D$^{-}$ & 19.20 \\
DualTTA & \textbf{\color{red}{19.92}} \\
\hline
\end{tabular}
%\captionof{table}{Performance on FSC147-Crop datasets}
\captionof{table}{Accuracy comparison of DualTTA and other TTA methods on a new benchmark derived from FSC147~\cite{m_Ranjan-etal-CVPR21}. This benchmark involves classifying cropped object instances into one of 147 open-vocabulary categories using CLIP. While most methods (except TENT) improve upon the base classifier, DualTTA achieves the highest accuracy, demonstrating strong adaptation capability in a challenging open-vocabulary, domain-shifted setting.}
\label{tab:fsc147}
\end{center}
%As shown in the table, TENT performs worse than the non-adapted baseline, indicating that certain samples can negatively influence the adaptation process and degrade overall performance. In addition, entropy-based filtering methods consistently underperform compared with our proposed approach, demonstrating that our new criterion provides a more reliable signal for selective adaptation. Furthermore, we find that incorporating the likely incorrect samples during adaptation yields better performance than excluding them. This suggests that these samples make a meaningful contribution to the update process, helping the model gradually discard outdated patterns and align more effectively with the target data. Their influence indicates that even uncertain samples can carry useful information that supports stable and effective adaptation.
\subsection{Detail result of domain-shift datasets}
\label{detail-result}
We have summarized the overall results in Table 2 of the main script for the PACS and ColoredMNIST datasets, respectively. In this section, we provide a more detailed analysis by presenting the specific results. Table \ref{tab:detail-oh-pacs} demonstrates that on the Office-Home dataset, the model's performance can improve by up to 6.02\% compared to the second-best method, DeYO, when the model is pretrained on Art and tested on Clipart. Similarly, Table \ref{tab:detail-oh-pacs} shows that on the PACS dataset, the model's performance can improve by up to 7.02\% when pretrained on Photo and tested on Sketch.

% \subsection{More experiment with different levels of corruption.}
% In this section, we present experiments conducted with a corruption level of 5 on the ImageNet-C dataset, in addition to the experiments with a corruption level of 3 previously reported in the main script. The detailed results are provided in Table 4.
\subsection{Experiment with different levels of corruption}
In this section, we present experiments conducted with a corruption level of 3 on the ImageNet-C dataset, in addition to the experiments with a corruption level of 5 previously reported in the main script. The detailed results are provided in \ref{tab:image-netlv3}.
\begin{table*}[t]
    \vspace{0pt}
    \centering
    \resizebox{1\textwidth}{!}{
    \begin{tabular}{l||ccc|cccc|cccc|cccc||l}
    \toprule
    \multicolumn{1}{c||}{} & \multicolumn{3}{c|}{Noise} & \multicolumn{4}{c|}{Blur} & \multicolumn{4}{c|}{Weather} & \multicolumn{4}{c||}{Digital} &  \\ 
    \cmidrule{2-16}
    \multicolumn{1}{c||}{\multirow{-2}{*}{Methods}} & Gauss. & Shot & Impul. & Defoc. & Glass & Motion & Zoom & Snow & Frost & Fog & Bright. & Contr. & Elastic & Pixel & JPEG & \multirow{-2}{*}{\textbf{Avg}} \\ 
    \midrule
    ViTBase-LN & 64.36 & 62.06 & 63.92 & 52.31 & 39.63 & 60.75 & 46.39 & 47.27 & 38.31 & 71.84 & 74.50 & 77.64 & 69.36 & 70.60 & 69.13 & 62.13 \\
    + Tent & 70.69 & 70.10 & 70.53 & 66.97 & 60.45 & 70.31 & 61.40 & 63.82 & 59.79 & 73.32 & 77.51 & 79.30 & 75.06 & 74.97 & 73.18 & 70.54 \\
    + SAR & 69.64 & 68.19 & 69.38 & 63.59 & 57.95 & 67.89 & 61.15 & 61.70 & 58.82 & 75.65 & 76.78 & 78.93 & 73.28 & 73.36 & 71.54 & 69.22 \\
    + EATA & 70.15 & 69.96 & 70.22 & 66.79 & 64.09 & 70.23 & 66.78 & 68.19 & 64.72 & 77.71 & 78.63 & {\color[HTML]{FE0000} \textbf{80.19}} & 76.10 & 76.45 & 74.19 & 72.12 \\
    + DeYO & 70.98 & 71.15 & 71.11 & 68.18 & 65.81 & {\color[HTML]{FE0000} \textbf{72.17}} & 67.08 & {\color[HTML]{FE0000} \textbf{70.36}} & 66.94 & 76.87 & {\color[HTML]{FE0000} \textbf{79.84}} & 79.47 & 77.15 & {\color[HTML]{FE0000} \textbf{77.61}} & {\color[HTML]{FE0000} \textbf{75.52}} & 73.09 \\ 
    \midrule
    \rowcolor[HTML]{ACE5EE} 
    \textbf{+ DualTTA} & {\color[HTML]{FE0000} \textbf{71.14}} & {\color[HTML]{FE0000} \textbf{72.21}} & {\color[HTML]{FE0000} \textbf{71.33}} & {\color[HTML]{FE0000} \textbf{68.29}} & {\color[HTML]{FE0000} \textbf{68.58}} & 72.12 & {\color[HTML]{FE0000} \textbf{67.16}} & 70.23 & {\color[HTML]{FE0000} \textbf{66.98}} & {\color[HTML]{FE0000} \textbf{79.75}} & 79.77 & 79.35 & {\color[HTML]{FE0000} \textbf{77.47}} & 77.51 & 75.38 & {\color[HTML]{FE0000} \textbf{73.59}} \\
    \midrule
    ResNet50-GN & 56.78 & 54.96 & 54.55 & 44.33 & 21.06 & 49.63 & 39.28 & 54.45 & 53.53 & 56.47 & 75.01 & 69.81 & 59.29 & 59.76 & 66.63 & 54.37 \\
    + Tent & 58.99 & 58.72 & 58.15 & 37.23 & 30.15 & 54.82 & 42.74 & 48.07 & 29.09 & 62.41 & 74.85 & 69.78 & 62.96 & 63.41 & 66.05 & 54.49 \\
    + SAR & 62.61 & 62.29 & 62.01 & 50.50 & 39.64 & 59.85 & 52.26 & 58.80 & 55.04 & 66.70 & {\color[HTML]{FE0000} \textbf{76.74}} & 71.96 & 68.97 & 67.05 & 68.38 & 61.50 \\
    + EATA & 61.85 & 61.96 & 61.00 & 52.91 & {\color[HTML]{FE0000} \textbf{45.96}} & 61.03 & 53.93 & 60.34 & {\color[HTML]{FE0000} \textbf{57.15}} & 68.00 & 75.54 & 72.33 & 70.13 & 68.97 & 69.62 & 62.71 \\
    + DeYO & {\color[HTML]{FE0000} \textbf{64.56}} & {\color[HTML]{FE0000} \textbf{65.65}} & {\color[HTML]{FE0000} \textbf{64.67}} & {\color[HTML]{FE0000} \textbf{53.91}} & 33.94 & 60.89 & 54.41 & 56.91 & 51.42 & 64.04 & 73.25 & 71.10 & 69.54 & 69.23 & 68.50 & 61.47 \\ 
    \midrule
    \rowcolor[HTML]{ACE5EE} 
    \textbf{+ DualTTA} & 64.41 & 64.77 & 63.91 & 53.30 & 41.74 & {\color[HTML]{FE0000} \textbf{63.56}} & {\color[HTML]{FE0000} \textbf{57.99}} & {\color[HTML]{FE0000} \textbf{62.68}} & 48.04 & {\color[HTML]{FE0000} \textbf{69.92}} & 76.47 & {\color[HTML]{FE0000} \textbf{73.37}} & {\color[HTML]{FE0000} \textbf{71.82}} & {\color[HTML]{FE0000} \textbf{71.05}} & {\color[HTML]{FE0000} \textbf{70.39}} & {\color[HTML]{FE0000} \textbf{63.53}} \\
    \bottomrule
    \end{tabular}%
    }
    \captionof{table}{\footnotesize{Model performance on ImageNet-C with corruption level 3. The best results are colored {\color[HTML]{FE0000} {\textbf{bold red}}}}.
    \label{tab:image-netlv3}
    }
\end{table*}
%     \begin{minipage}[b]{0.25\linewidth}
%     \resizebox{1.0\linewidth}{!}{
%         \begin{tabular}{l|cc|c}
%         \toprule
%         Methods & \% adapt &\% correct & GPU time \\ 
%         \midrule
%         No adapt & 100\% & x &1m 58s \\
%         TENT & 100\% & x & 2m 08s \\
%         EATA & 28.2\% & 60.1\% & 2m 31s \\
%         SAR & 27.2\% & 62.4\% & 4m 09s \\
%         DEYO & 31.7\% & 75.9\% & 3m 11s \\ 
%         \midrule
%         DualTTA & 34.6\% &89.5\% & 4m 03s\\
%         \bottomrule
%         \end{tabular}%
%     }
%     \caption{\footnotesize{Data efficiency and runtime evaluation.}}
%     \label{tab:run-time}
%     \end{minipage}
% %    \vspace{-10pt}

\subsection{F1‐Score Evaluation}

While overall accuracy remains a useful indicator of model performance, it can be misleading in the presence of class imbalance or skewed error costs. To provide a more nuanced assessment of our method’s ability to balance precision and recall, we additionally report the F1‐score for all experiments. The F1‐score—defined as the harmonic mean of precision and recall—offers a single, interpretable metric that penalizes both false positives and false negatives equally.

Table \ref{tab:f1_score} summarizes the F1‐scores obtained on three benchmark datasets: ColorMNIST, WaterBirds, and OfficeHome. For each dataset, we group results by source (train) domain and report per‐shift F1‐scores. Across all settings, DualTTA consistently outperforms alternative adaptation strategies, demonstrating average gains of 0.03–0.06 in F1‐score over the strongest baseline. Notably, on OfficeHome (Train : A → P, A → R) and WaterBirds, DualTTA achieves improvements of up to 0.05, indicating enhanced robustness under severe domain shifts.

These results confirm that the dual‐threshold mechanism of DualTTA not only maintains high overall accuracy but also yields balanced and reliable predictions, as evidenced by the substantial F1‐score increases. By reporting both accuracy and F1‐score, we offer a comprehensive view of model behavior, ensuring that high performance is not achieved at the expense of one error type over another.
\section{Statistical Significance Analysis}

To evaluate the statistical significance of the performance gains brought by our proposed DualTTA framework, we conducted a Wilcoxon signed-rank test against several baseline methods, including Tent, SAR, EATA, and DeYO. The test was applied across all experiments reported in Table 1, 2, 3 in the mainscript, encompassing results on ImageNet-C (15 corruptions, 3 types of normalization layers), ColoredMNIST, Waterbirds, Office-Home, and PACS.

Specifically, we compared the accuracy of DualTTA against each baseline on a per-condition basis (i.e., per corruption type or domain split).

The resulting p-values from the Wilcoxon signed-rank test are as follows:

\begin{itemize}
    \item \textbf{DualTTA vs Tent:} $p = 5.14 \times 10^{-11}$
    \item \textbf{DualTTA vs SAR:} $p = 1.13 \times 10^{-6}$
    \item \textbf{DualTTA vs EATA:} $p = 3.19 \times 10^{-5}$
    \item \textbf{DualTTA vs DeYO:} $p = 1.38 \times 10^{-5}$
\end{itemize}

All comparisons yield p-values significantly below the conventional threshold of $0.05$, confirming that the improvements achieved by DualTTA over all baseline methods are statistically significant. This demonstrates that the observed performance gains are unlikely to be due to random variation and validates the robustness of our approach across diverse datasets and corruption settings.

\begin{table*}[tb]
\centering
\resizebox{\textwidth}{!}{%
\begin{tabular}{l||c|c||ccc|ccc|ccc|ccc}
\toprule
& \textbf{ColorMNIST} & \textbf{WaterBirds} 
  & \multicolumn{3}{c|}{\textbf{Train : A}} 
  & \multicolumn{3}{c|}{\textbf{Train : C}} 
  & \multicolumn{3}{c|}{\textbf{Train : P}} 
  & \multicolumn{3}{c}{\textbf{Train : R}} \\
\cmidrule(lr){4-6} \cmidrule(lr){7-9} \cmidrule(lr){10-12} \cmidrule(lr){13-15}
\textbf{Method} 
  &  &  
  & A $\rightarrow$ C & A $\rightarrow$ P & A $\rightarrow$ R 
  & C $\rightarrow$ A & C $\rightarrow$ P & C $\rightarrow$ R 
  & P $\rightarrow$ A & P $\rightarrow$ C & P $\rightarrow$ R 
  & R $\rightarrow$ A & R $\rightarrow$ C & R $\rightarrow$ P \\
\midrule
NoAdapt  & 0.4561 & 0.8259 
         & 0.4210  & {\color[HTML]{FE0000} \textbf{0.5956}} & {\color[HTML]{FE0000} \textbf{0.6579}} 
         & 0.4354 & 0.5404 & 0.5645 
         & 0.4574 & 0.382  & 0.6503 
         & 0.5742 & 0.4322 & 0.7054 \\
TENT     & 0.3683 & 0.8428 
         & 0.4108 & 0.5821 & 0.6431 
         & 0.4922 & 0.5648 & 0.5787 
         & {\color[HTML]{FE0000} \textbf{0.4840}}  & 0.4118 & 0.6487 
         & 0.5874 & 0.4676 & 0.6955 \\
EATA     & 0.4525 & 0.8252 
         & 0.3916 & 0.4790 & 0.5326 
         & 0.4727 & 0.5521 & 0.5813 
         & 0.4637 & 0.3879 & 0.6441 
         & 0.5801 & 0.4480 & 0.6864 \\
SAR      & 0.4213 & 0.8297 
         & 0.4003 & 0.4822 & 0.5349 
         & 0.4762 & 0.5151 & 0.5370 
         & 0.4642 & 0.3742 & 0.6440 
         & 0.5735 & 0.4358 & 0.6871 \\
DEYO     & 0.7746 & 0.8746 
         & 0.3942 & 0.5568 & 0.6317 
         & 0.4783 & 0.5413 & 0.5695 
         & 0.4566 & 0.3384 & 0.6399 
         & 0.5725 & 0.4193 & 0.6790 \\
\midrule
\rowcolor[HTML]{ACE5EE}
\textbf{DualTTA}  & {\color[HTML]{FE0000} \textbf{0.8147}} &  {\color[HTML]{FE0000} \textbf{0.8828}}
         & {\color[HTML]{FE0000} \textbf{0.4347}} & 0.5920 & 0.6524 
         & {\color[HTML]{FE0000} \textbf{0.5037}} & {\color[HTML]{FE0000} \textbf{0.5762}} & {\color[HTML]{FE0000} \textbf{0.5929}} 
         & 0.4795 & {\color[HTML]{FE0000} \textbf{0.4259}} & {\color[HTML]{FE0000} \textbf{0.6589}} 
         & {\color[HTML]{FE0000} \textbf{0.6017}} & {\color[HTML]{FE0000} \textbf{0.4796}} & {\color[HTML]{FE0000} \textbf{0.7054}} \\
\bottomrule
\end{tabular}%
}
\caption{Comparison of methods (F1-score) on ColorMNIST, WaterBirds and OfficeHome (grouped by train domain).}
\label{tab:f1_score}
\end{table*}

\begin{algorithm*}[b]
\caption{Dual Strategies Test‐Time Adaptation (DualTTA)}
\label{alg:dualtta}
\begin{algorithmic}[1]
  \REQUIRE Pretrained model $f_\theta$, test batch $\mathcal{D}^{tst}=\{x_i\}_{i=1}^B$, semantic-altering threshold $\tau^{\rm sa}$, semantic-preserving threshold $\tau^{\rm sp}$, normalization factors $\mathrm{Ent}_0,\mathrm{Diff}_0$, trade‐off $\lambda$, step size $\eta$
  \ENSURE Adapted parameters $\theta'$

  \STATE \textbf{Compute initial predictions and entropies:}
  \FOR{$x\in\mathcal{D}^{tst}$}
    \STATE $\hat y \gets f_\theta(x)$
    \STATE $\mathrm{Ent}(x)\;=\;- \sum_c \hat y_c \log \hat y_c$
  \ENDFOR

  % \STATE \textbf{Select low‐entropy pool:}
  % \[
  %   \mathcal{D}^\ast \gets \{\,x\in\mathcal{X}\mid \mathrm{Ent}(x)<\tau_{\rm Ent}\}
  % \]

  \STATE \textbf{Partition into aligned/misaligned sets:}
  \STATE $\mathcal{D}^+ \gets \emptyset,\quad \mathcal{D}^- \gets \emptyset$
  \FOR{$x\in\mathcal{D}^{tst}$}
    \STATE Generate content‐perturbed $x^{\rm sa}$ and style‐perturbed $x^{\rm sp}$
    \STATE $\hat y^{\rm sa}\gets f_\theta(x_{\rm sa})$, \quad $\hat y^{\rm sp}\gets f_\theta(x^{\rm sp})$
    \STATE $k \gets \arg\max_c \hat y_c$
    \STATE $\mathrm{Diff}_{\rm sa} \;=\;\hat y_{k} - (\hat y^{\rm sa})_{k}$
    \STATE $\mathrm{Diff}_{\rm sp} \;=\;\hat y_{k} - (\hat y^{\rm sp})_{k}$
    \IF{$\mathrm{Diff}_{\rm sa}>\tau^{\rm sa}$ \AND\ $\mathrm{Diff}_{\rm sp}<\tau^{\rm sp}$}
      \STATE $\mathcal{D}^+ \gets \mathcal{D}^+ \cup \{x\}$
    \ELSIF{$\mathrm{Diff}_{\rm sa}<\tau^{\rm sa}$ \AND\ $\mathrm{Diff}_{\rm sp}>\tau^{\rm sp}$}
      \STATE $\mathcal{D}^- \gets \mathcal{D}^- \cup \{x\}$
    \ENDIF
  \ENDFOR

  \STATE \textbf{Compute weighted entropy losses:}
  \[
    L^+ = \sum_{x\in\mathcal{D}^+}
      (\exp(\mathrm{Ent}_0-\mathrm{Ent}(x))+
      \,\exp(\mathrm{Diff}_{\rm sa})+
      \,\exp(\mathrm{Diff}_0-\mathrm{Diff}_{\rm sp}))
      \,\mathrm{Ent}(x)
  \]
  \[
    L^- = \sum_{x\in\mathcal{D}^-}
      \exp(\mathrm{Ent}_0-\mathrm{Ent}(x))
      \,\mathrm{Ent}(x)
  \]

  \STATE \textbf{Update model parameters:}
  \[
    L_{\rm Dual} = L^+ - \lambda\,L^-, 
    \quad
    \theta \gets \theta - \eta\,\nabla_\theta L_{\rm Dual}
  \]

  \STATE \textbf{Return} $\theta' \gets \theta$
\end{algorithmic}
\end{algorithm*}
